# Supplementary material for: Advancing Multiple Instance Learning with Continual Learning for Whole Slide Imaging
Source: arXiv:2505.10649 source file (2025-05-15)
Supplement: Supplementary file 1 [file vis_suppl.pdf]

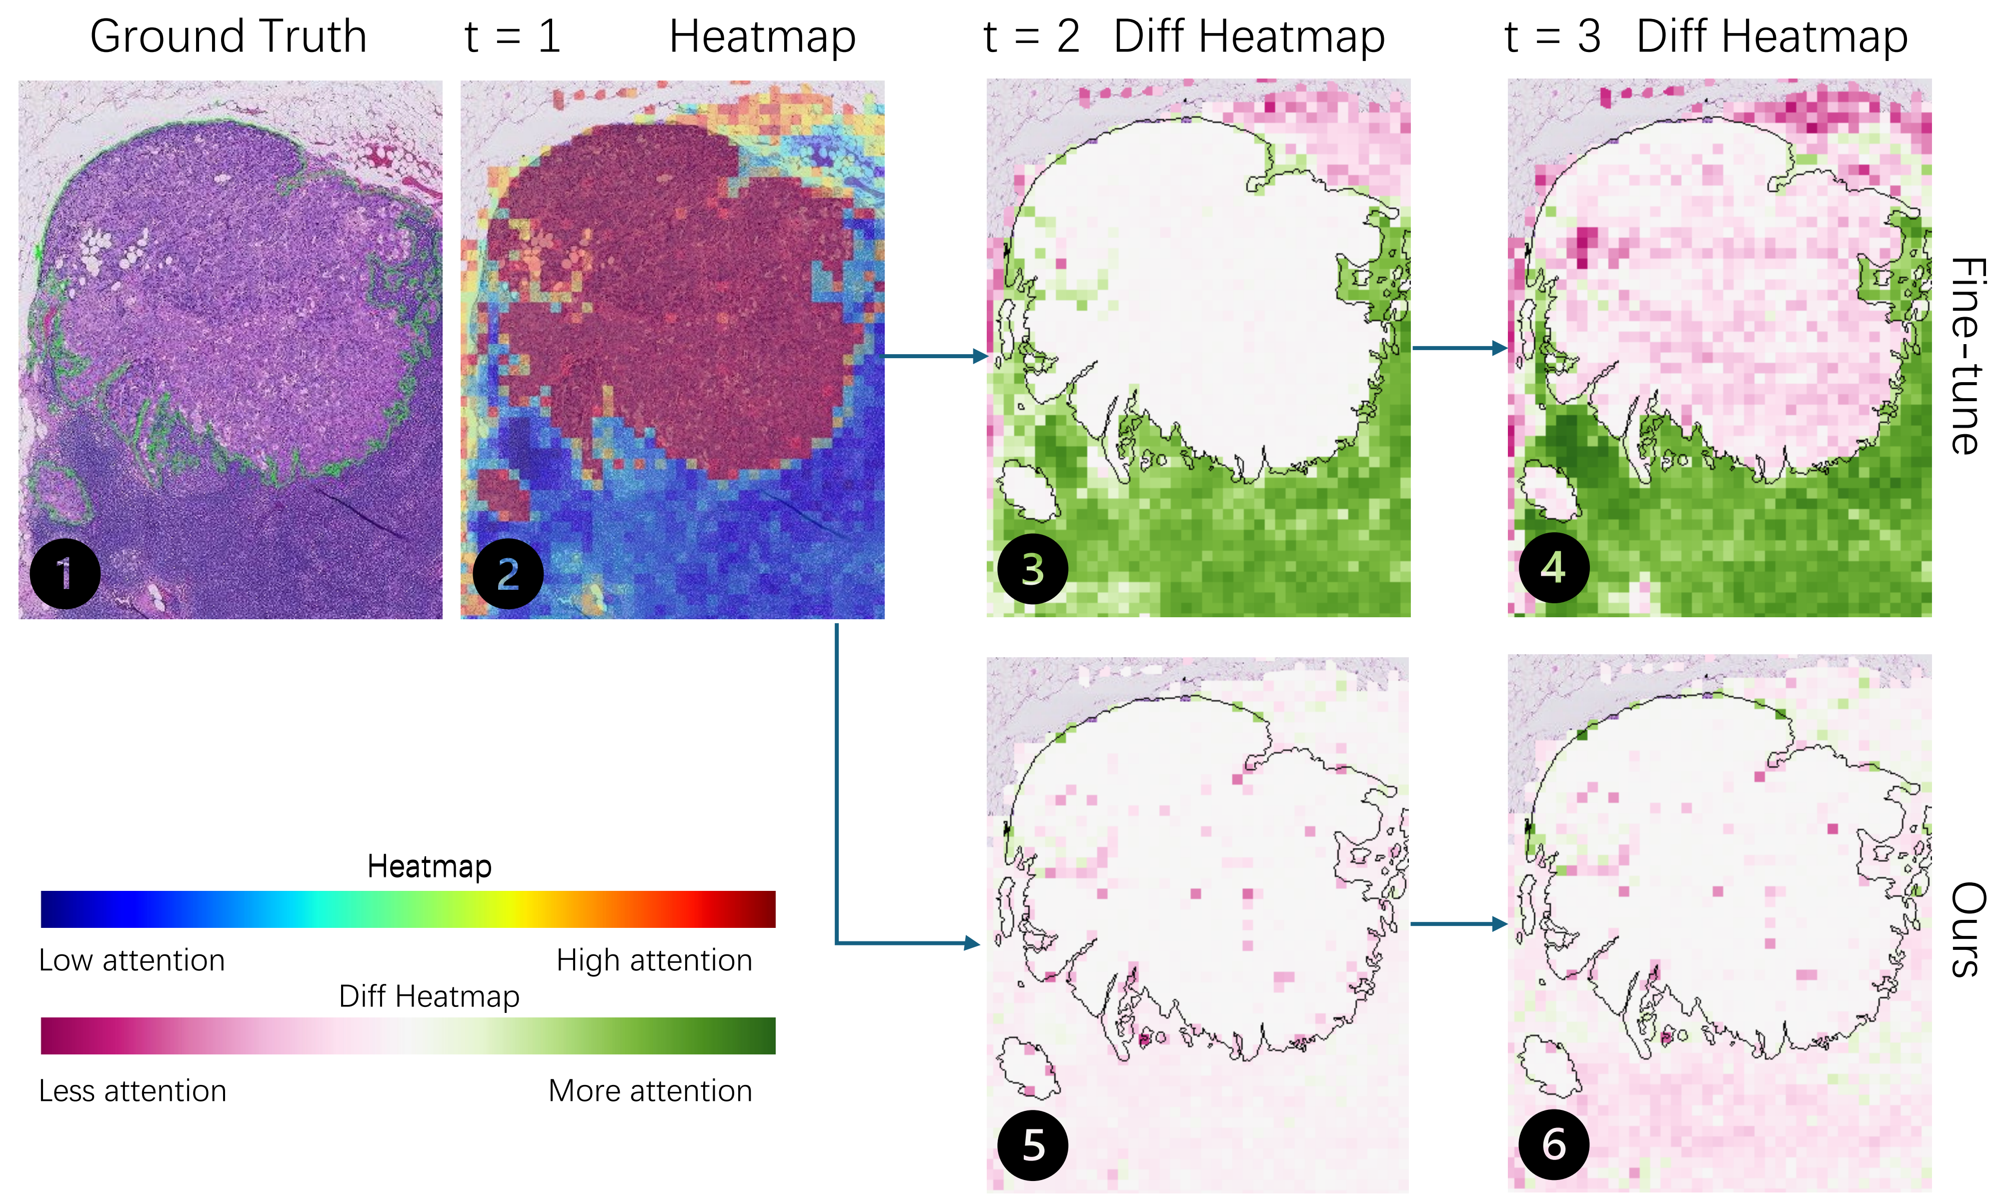
Ground Truth
t = 1
Heatmap
t = 2 Diff Heatmap
t = 3 Diff Heatmap
Fine-tune
Ours
1
2
3
4
5
6
Heatmap
Low attention
High attention
Diff Heatmap
Less attention
More attention

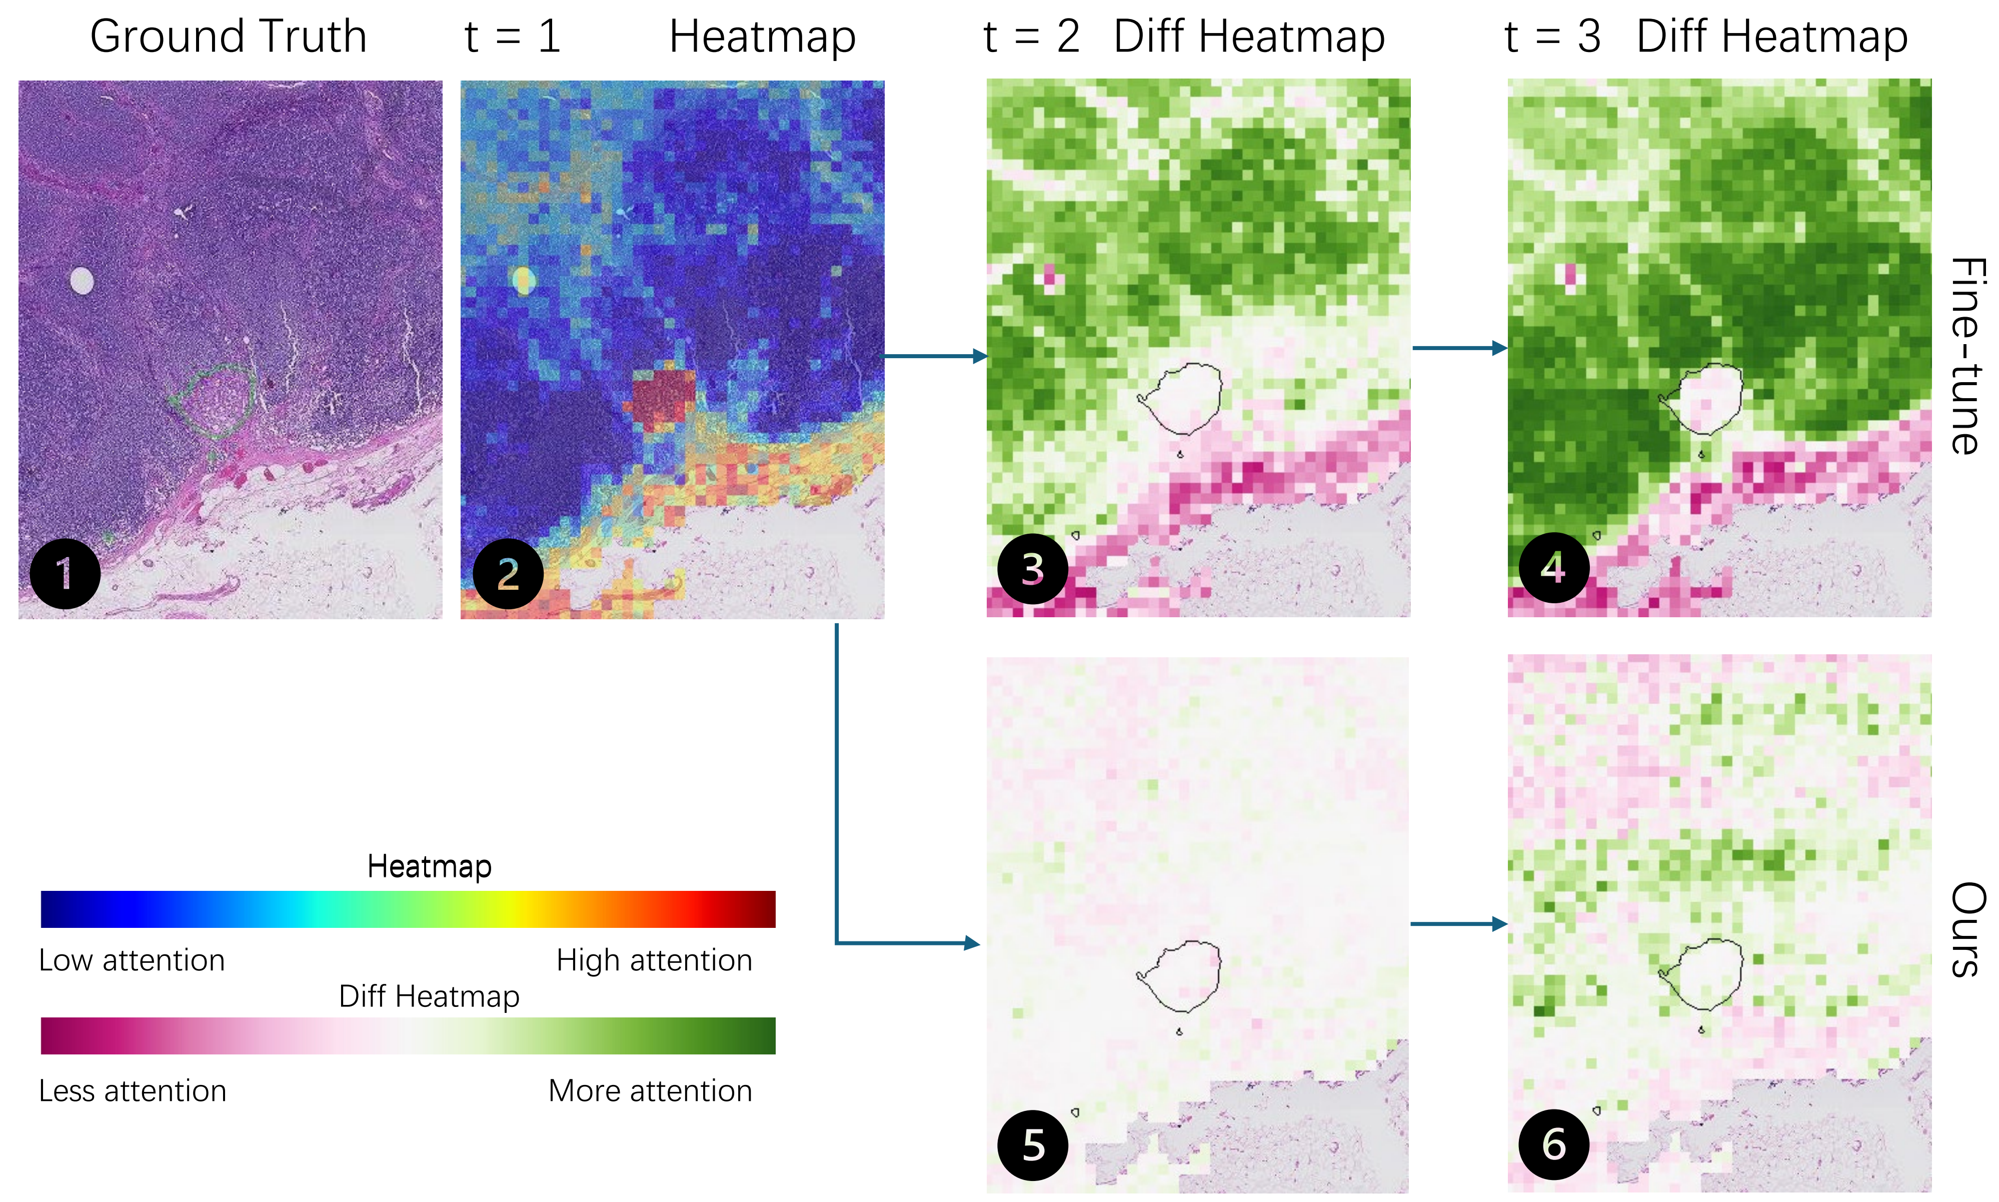
Ground Truth
t = 1
Heatmap
t = 2
Diff Heatmap
t = 3
Diff Heatmap
Fine-tune
Ours
1
2
3
4
5
6
Heatmap
Low attention
High attention
Diff Heatmap
Less attention
More attention

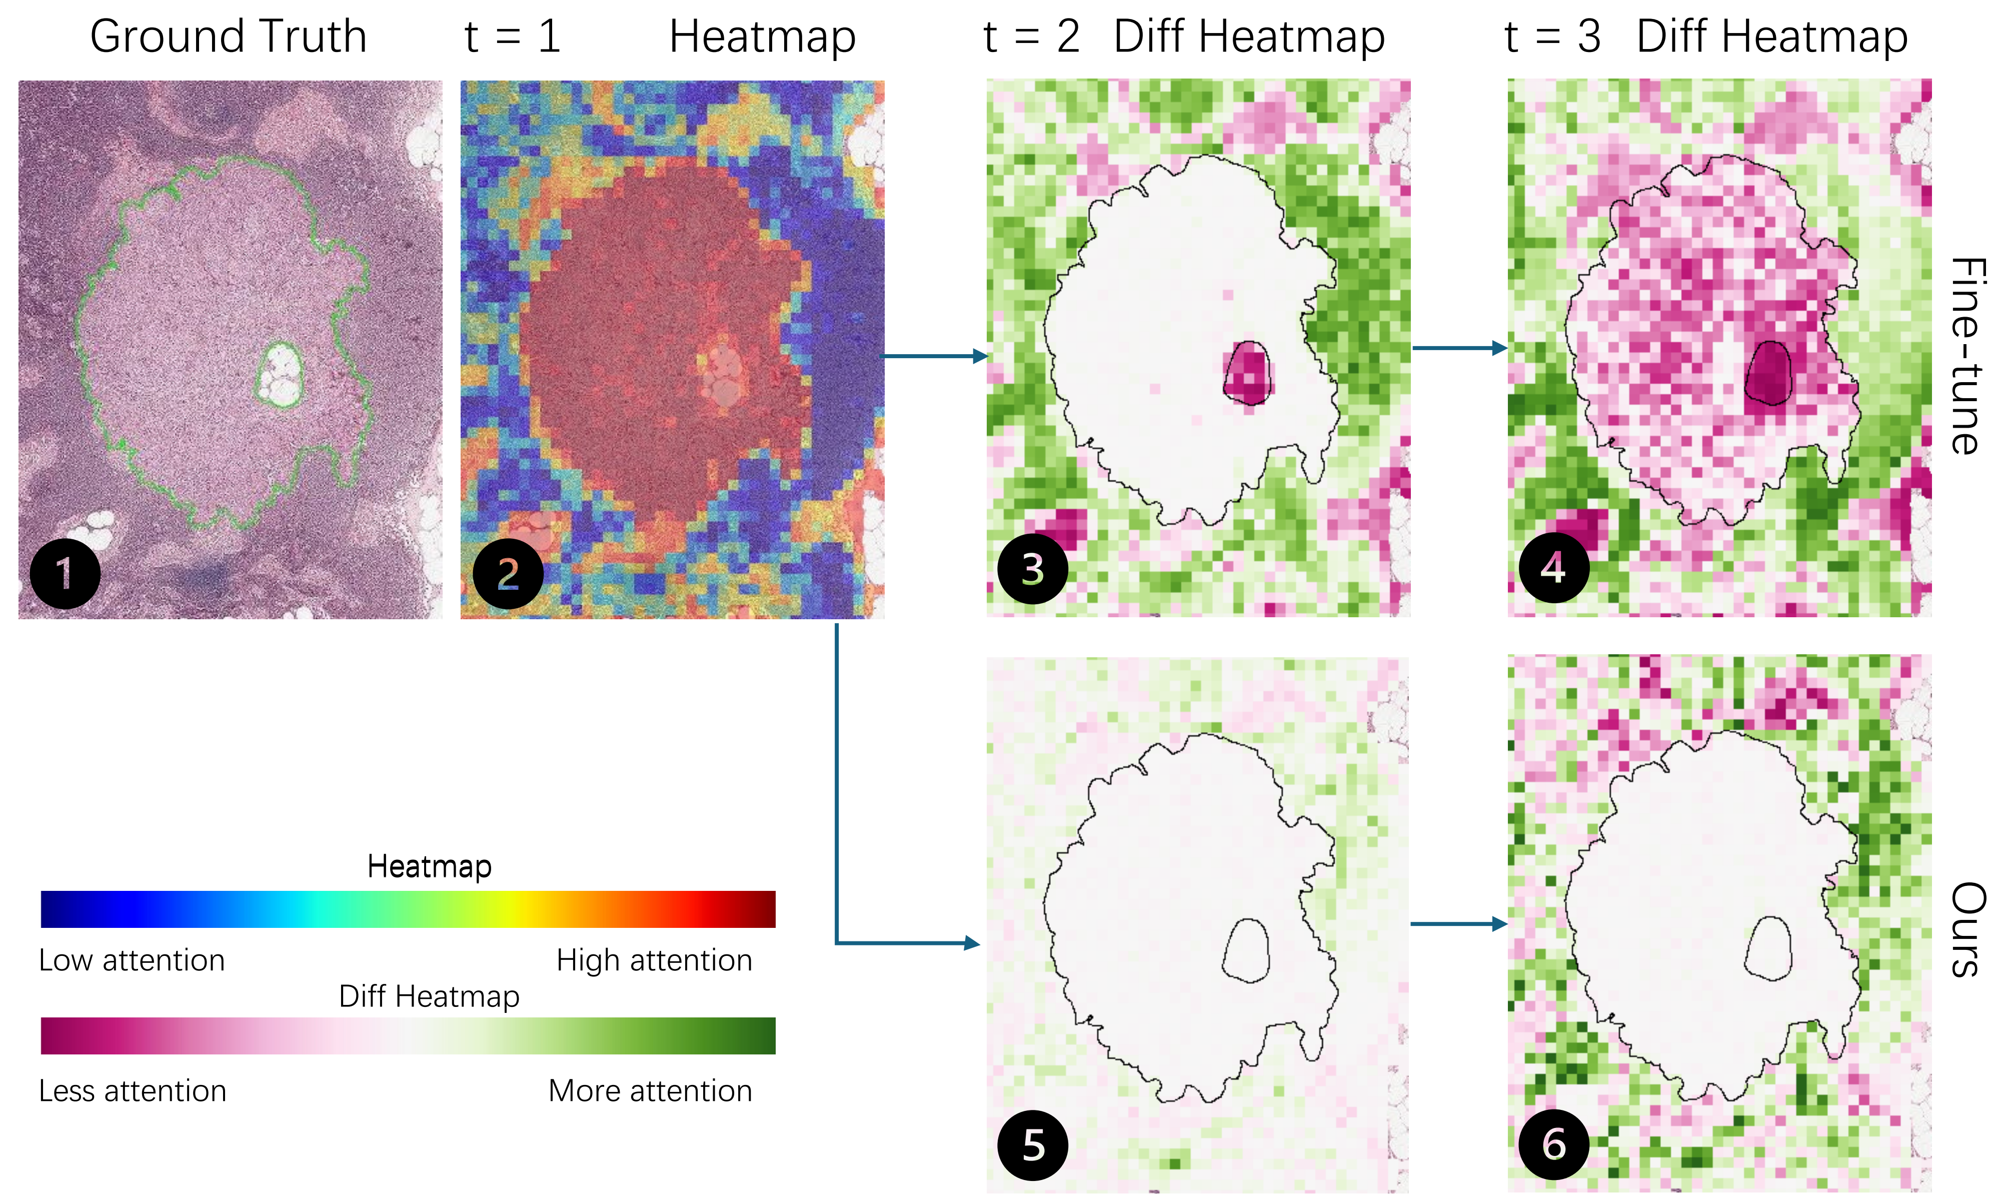

Ground Truth
t = 1
Heatmap
t = 2
Diff Heatmap
t = 3
Diff Heatmap
1
2
3
4
5
6
Fine-tune
Ours
Heatmap
Low attention
High attention
Diff Heatmap
Less attention
More attention

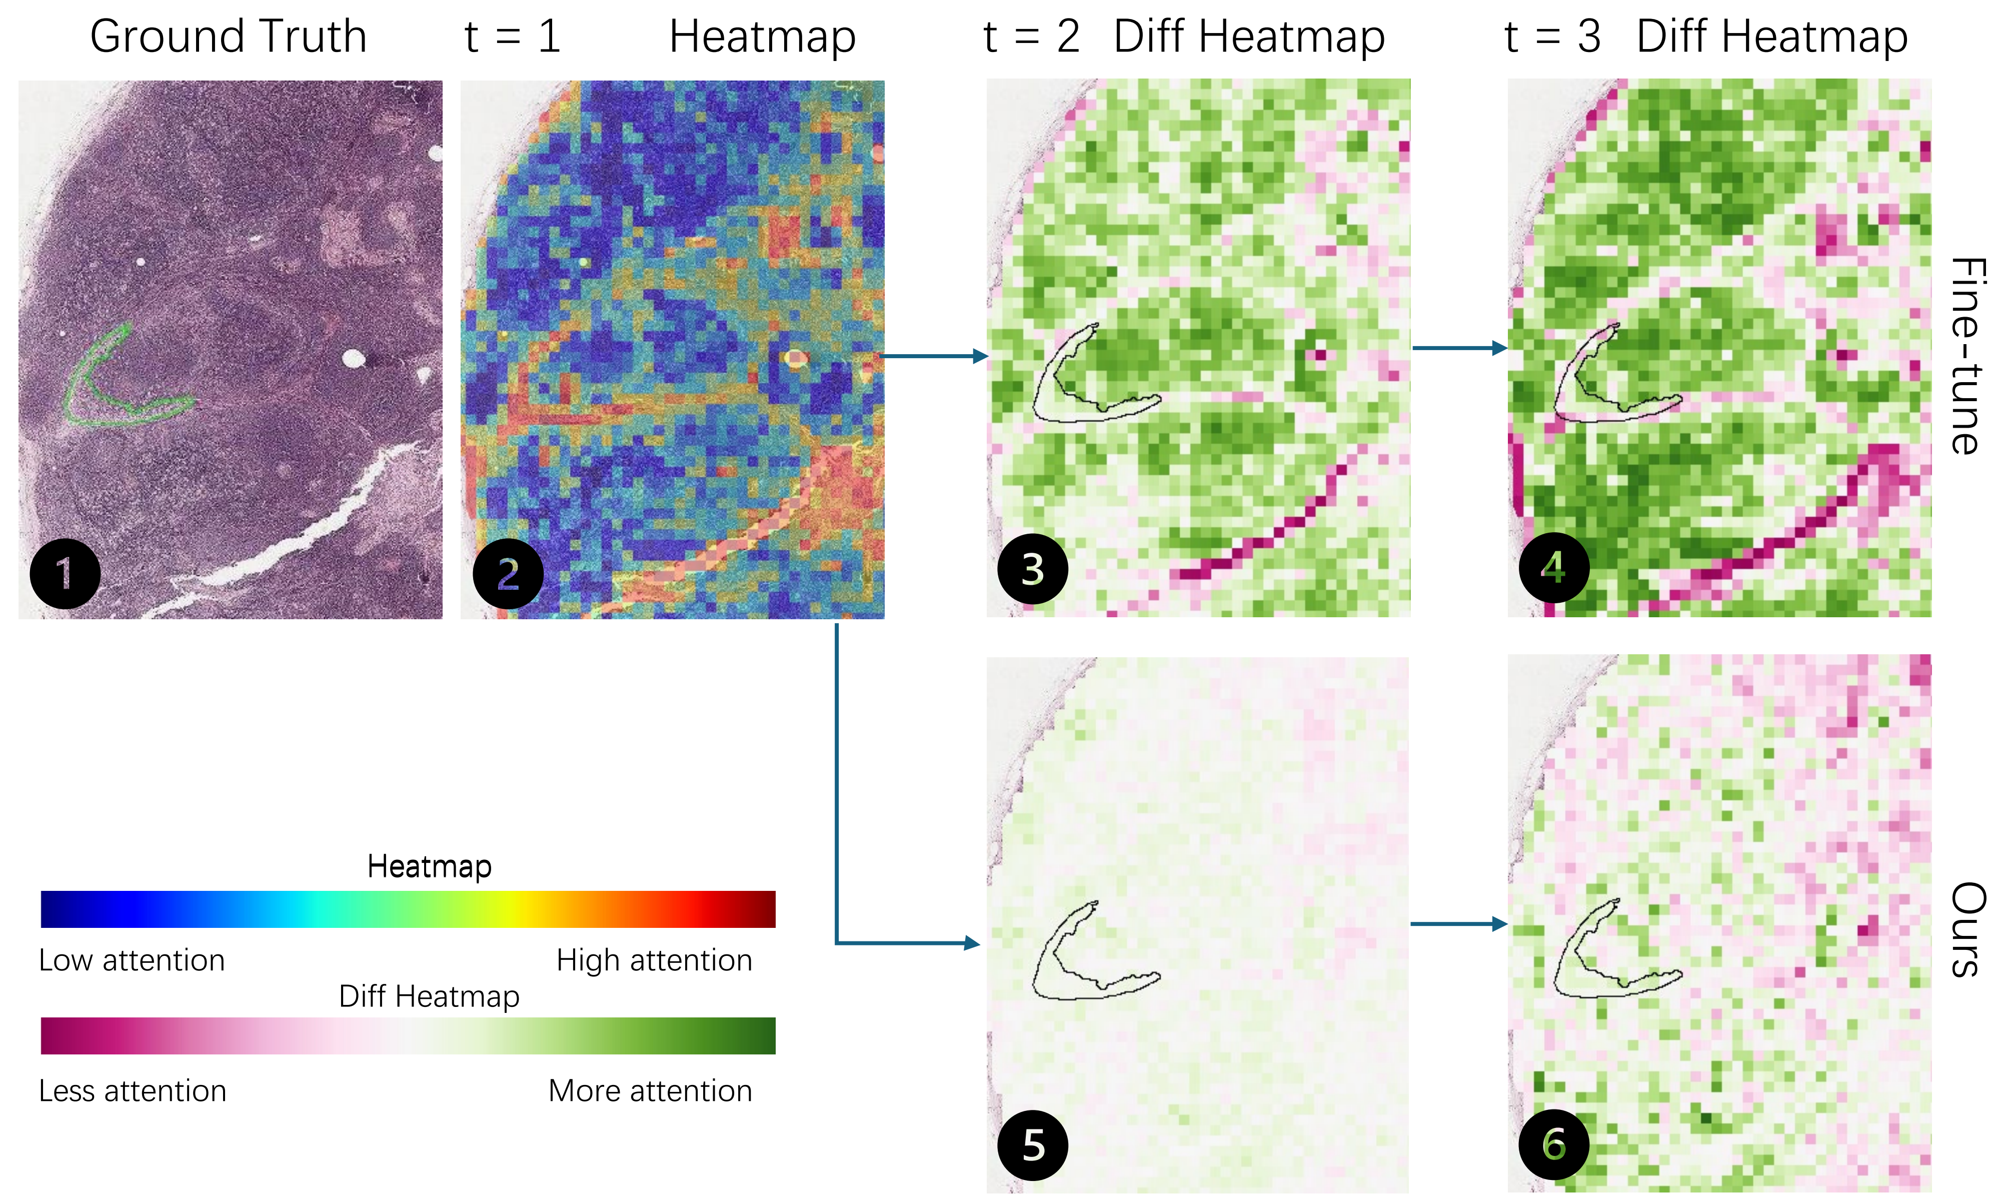

Ground Truth
t = 1 Heatmap
t = 2 Diff Heatmap
t = 3 Diff Heatmap
Fine-tune
Ours
1
2
3
4
5
6
Heatmap
Low attention
High attention
Diff Heatmap
Less attention
More attention

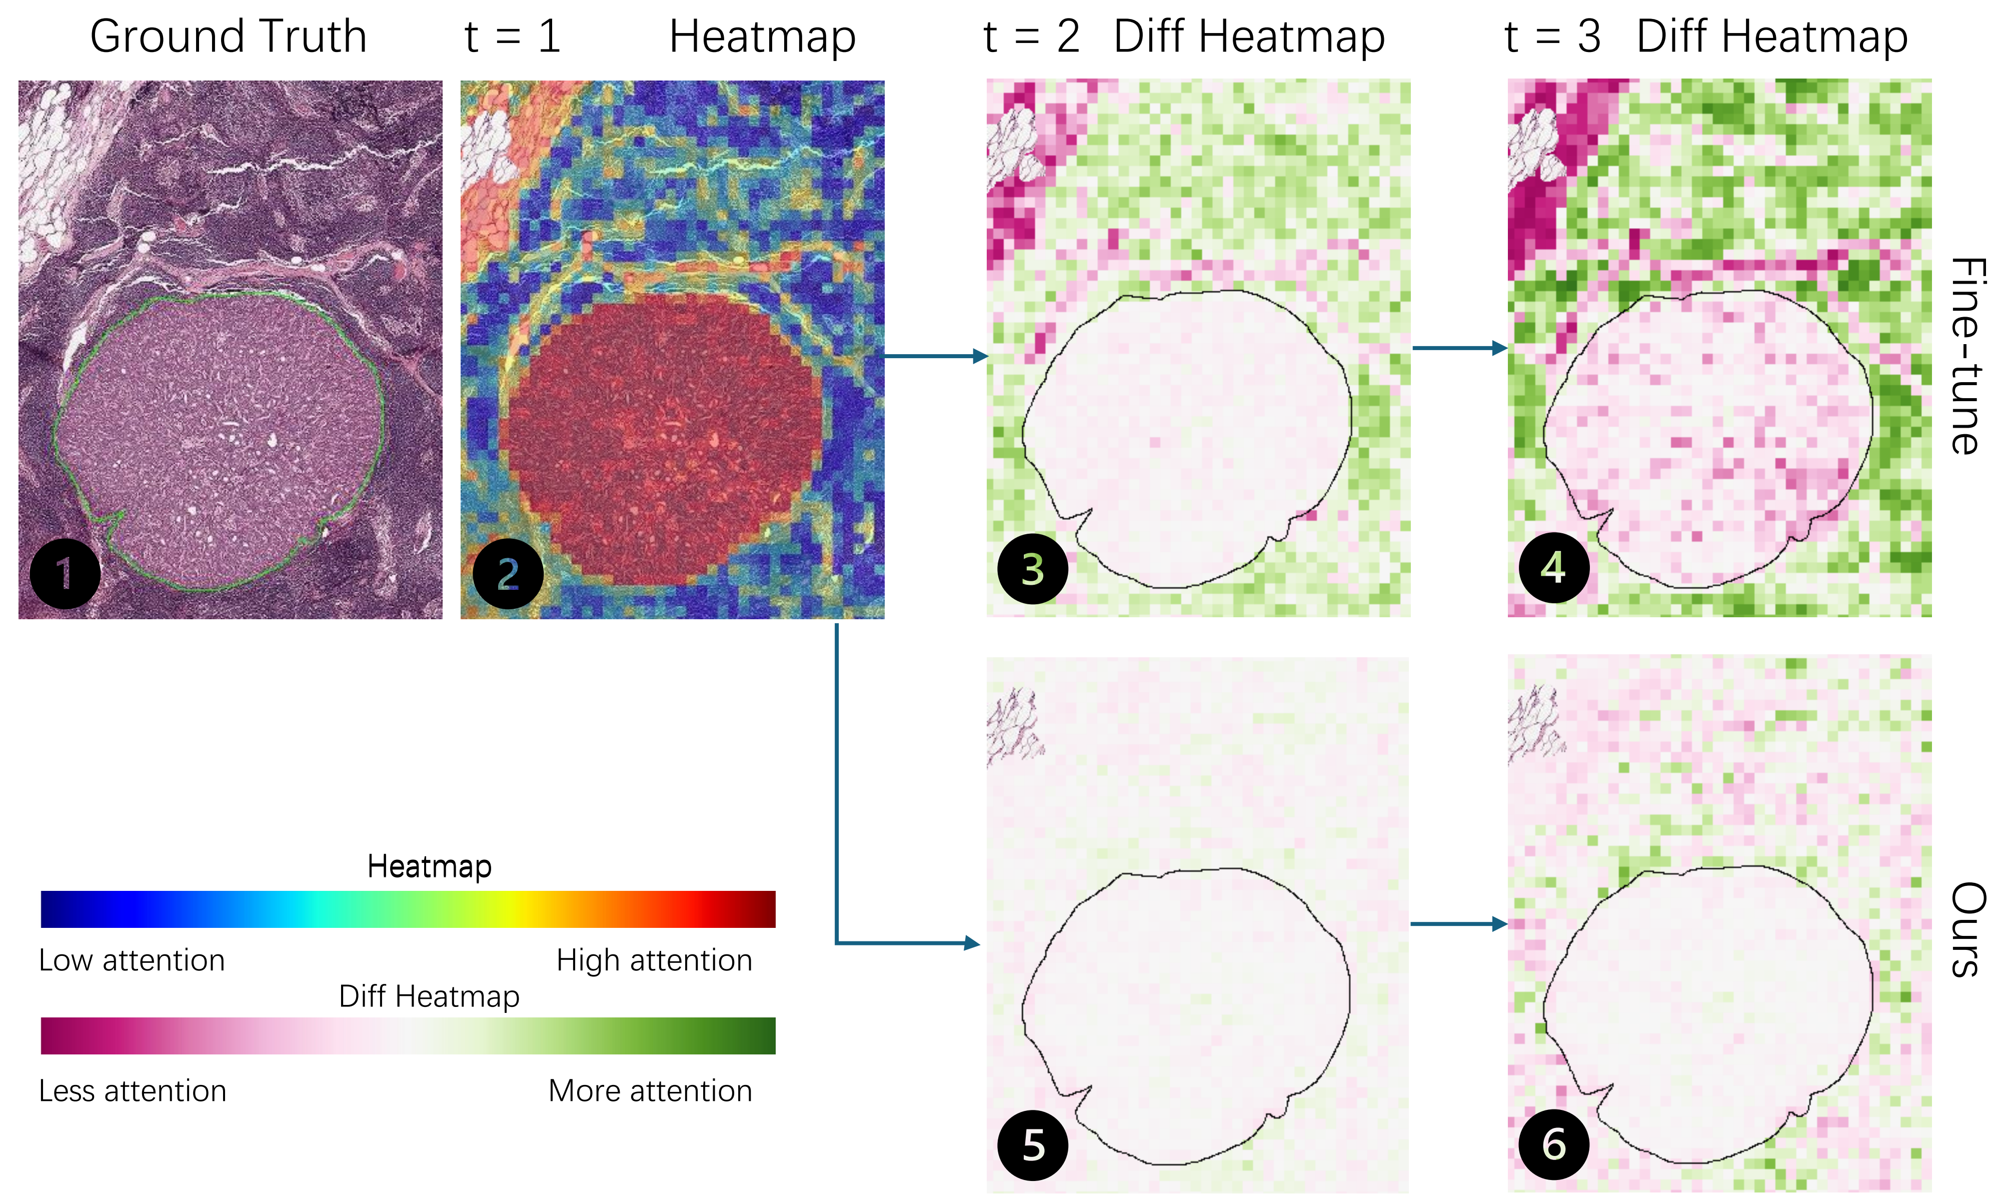

Ground Truth
t = 1 Heatmap
t = 2 Diff Heatmap
t = 3 Diff Heatmap
Fine-tune
Ours
1
2
3
4
5
6
Heatmap
Low attention
High attention
Diff Heatmap
Less attention
More attention

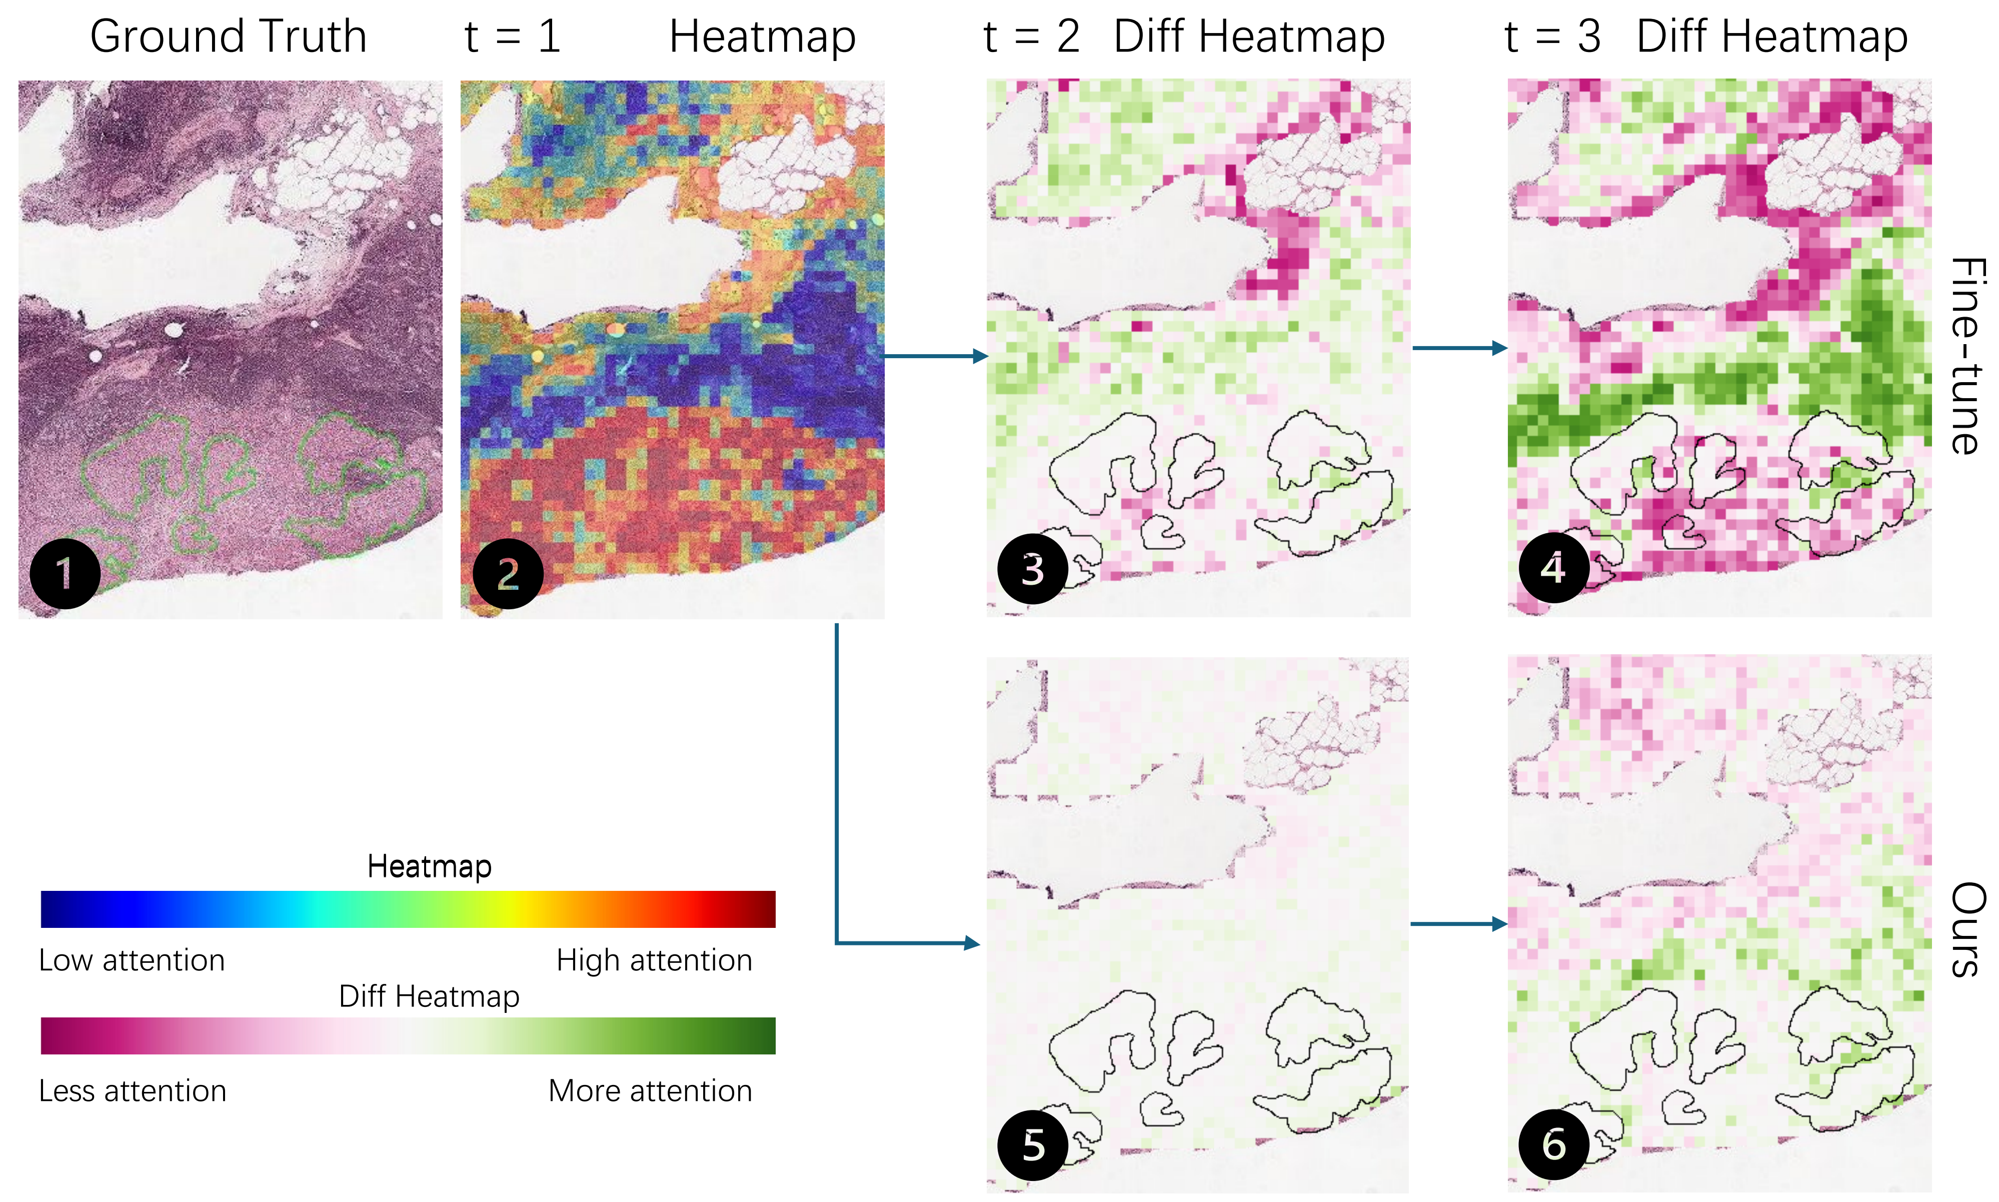
Ground Truth
t = 1
Heatmap
t = 2
Diff Heatmap
t = 3
Diff Heatmap
Fine-tune
Ours
1
2
3
4
5
6
Heatmap
Low attention
High attention
Diff Heatmap
Less attention
More attention

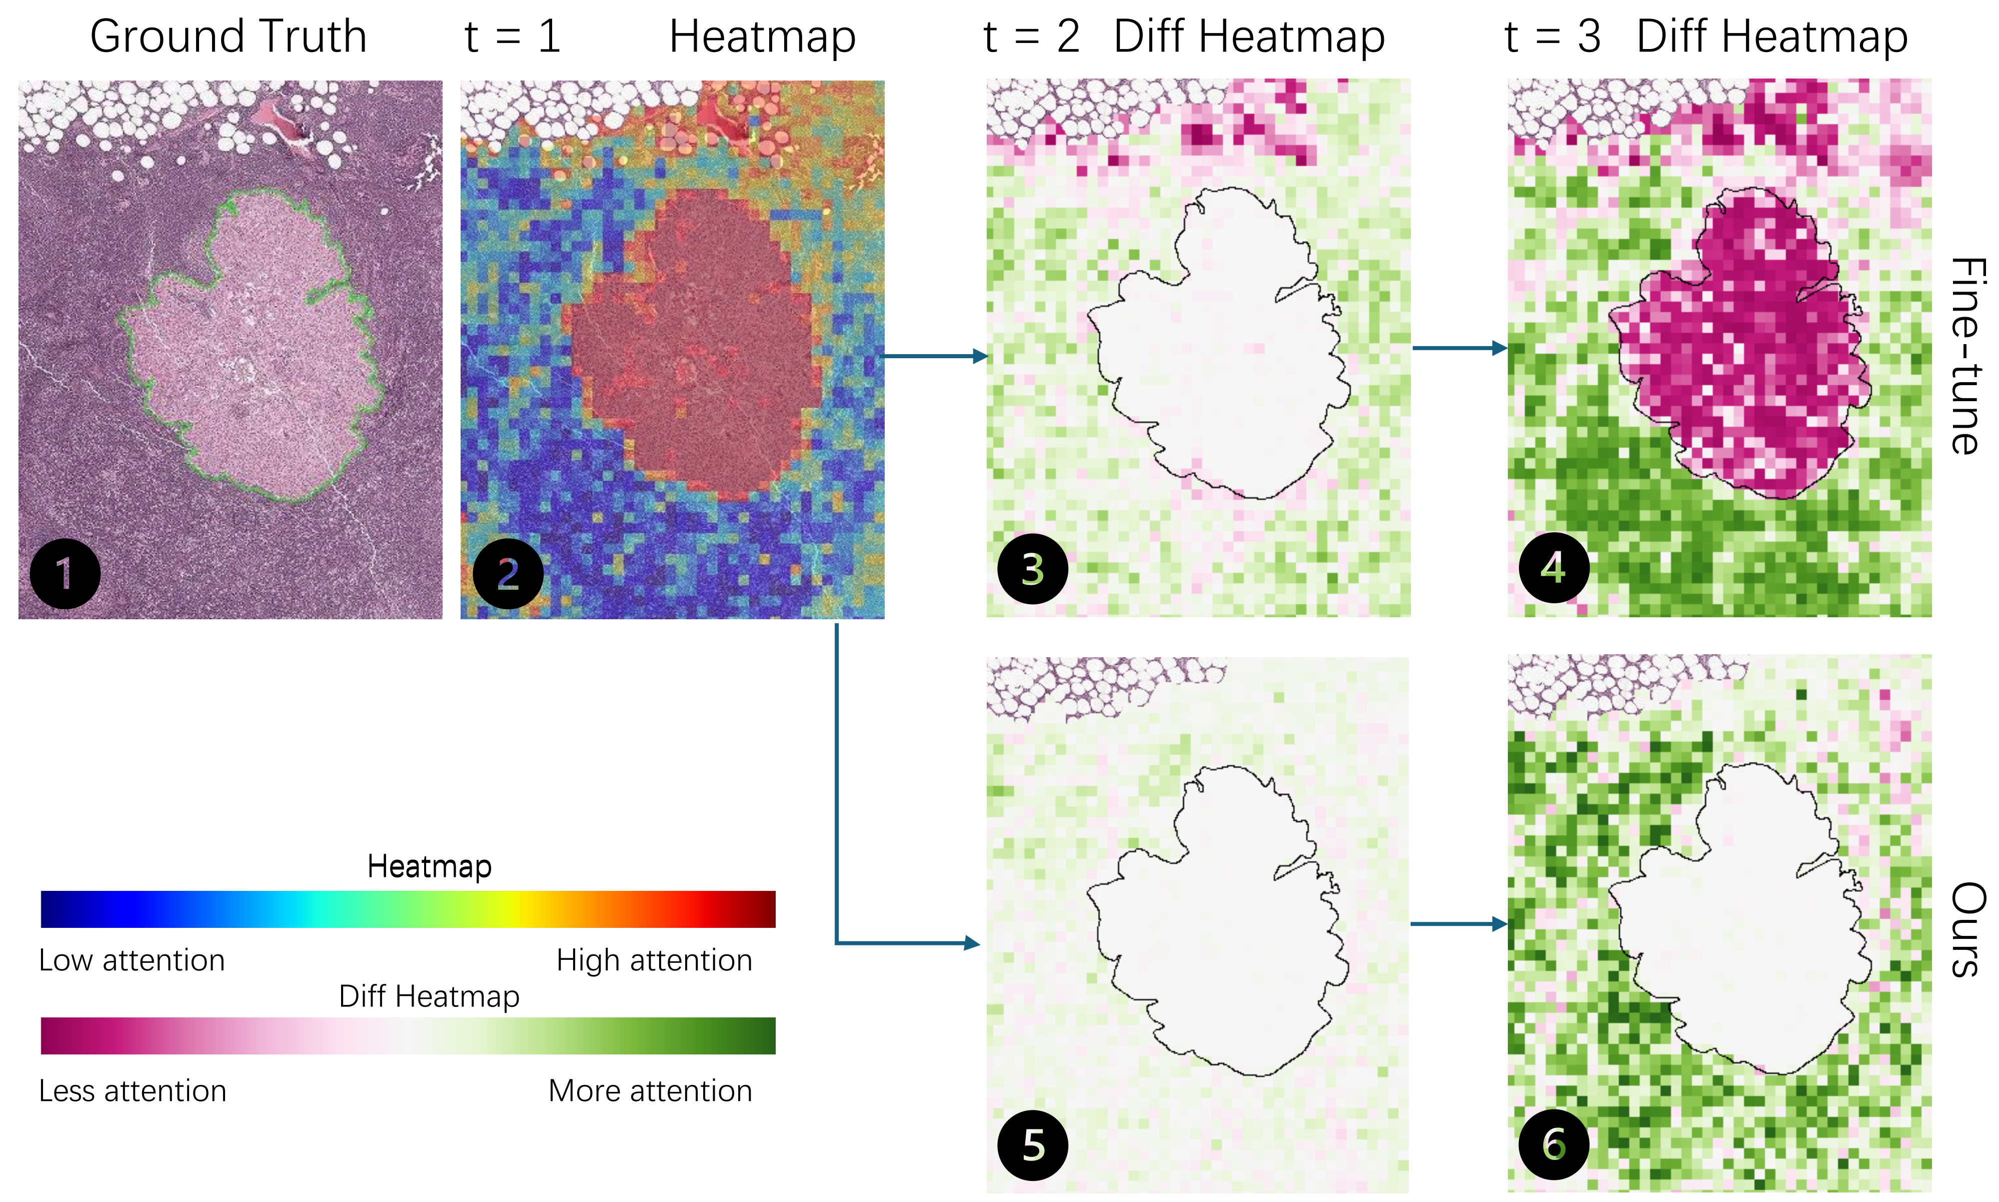
Ground Truth
t = 1
Heatmap
t = 2
Diff Heatmap
t = 3
Diff Heatmap
Fine-tune
Ours
1
2
3
4
5
6
Heatmap
Low attention
High attention
Diff Heatmap
Less attention
More attention
